# Supplementary material for: Is News Recommendation a Sequential Recommendation Task?
Source: arXiv:2108.08984 source file (2021-08-26)
Supplement: Supplementary file 1 [file supplement.tex]

\section{Appendix}

\subsection*{Experimental Environment}

Our experiments are conducted on a cloud Linux server with Ubuntu 16.04 operating system.
The codes are written in Python 3.6 using the Keras library 2.2.4 with Tensorflow 1.12 backend.
The GPU type is Nvidia Tesla V100 with 32GB GPU memory.
Each experiment is run by a single thread.

\subsection*{Hyperparameter Settings}

The detailed hyperparameter settings on each dataset used in this paper are listed in Table~\ref{hyper}.

\begin{table*}[t]
\resizebox{0.98\textwidth}{!}{
\begin{tabular}{lcccccc}
\hline
\multicolumn{1}{c}{Method}        & Amazon       & IMDB         & \begin{tabular}[c]{@{}c@{}}MIND\\ (classification)\end{tabular} & \begin{tabular}[c]{@{}c@{}}MIND\\ (recommendation)\end{tabular}              & CNN/DailyMail & PubMed       \\ \hline
\# Encoder Layer                  & 2            & 2            & 2                                                               & 1                                                                            & 4             & 2            \\
\# Decoder Layer                  & -            & -            & -                                                               & -                                                                            & 4             & 4            \\
\# Global Token                   & 8            & 8            & 16                                                              & 8                                                                            & 64            & 64           \\
\# Random Token                   & 8            & 8            & 16                                                              & 8                                                                            & 64            & 64           \\
Window size (Longformer, BigBird) & 8            & 8            & 16                                                              & 8                                                                            & 64            & 64           \\
Window size (Poolingformer)       & 64           & 64           & 256                                                             & 64                                                                           & 256           & 256          \\
Block length (BigBird)            & 4            & 4            & 8                                                               & 4                                                                            & 32            & 32           \\
Projection dimension (Linformer)  & 16           & 16           & 16                                                              & 16                                                                           & 64            & 64           \\
\# Attention Head                 & 16           & 16           & 16                                                              & 16                                                                           & 16            & 16           \\
Beam Size                         & -            & -            & -                                                               & -                                                                            & 5             & 5            \\
Hidden dimension                  & 256          & 256          & 256                                                             & 256                                                                          & 256           & 256          \\
Loss                              & Crossentropy & Crossentropy & Crossentropy                                                    & Crossentropy                                                                 & Crossentropy  & Crossentropy \\
Batch Size                        & 64           & 64           & 64                                                              & 64                                                                           & 32            & 32           \\
Optimizer                         & Adam         & Adam         & Adam                                                            & Adam                                                                         & Adam          & Adam         \\
Learning Rate                     & 1e-3         & 1e-3         & 1e-3                                                            & \begin{tabular}[c]{@{}c@{}}3e-6 for PLM-NR\\ 1e-4 for others\end{tabular} & 1e-4          & 1e-4         \\
Max Epochs                         & 3         & 3         & 3                                                            & 3                                                                         & 12          & 15         \\
Dropout                           &  0.2         & 0.2         & 0.2 & 0.2 & 0.2 & 0.2                                                                                                                                                                                              \\ \hline
\end{tabular}

}
\caption{Detailed hyperparameter settings on each dataset.}\label{hyper}
\end{table*}
